# Supplementary material for: Sensitivity Enhancement of (Hyper-)CEST Image Series by Exploiting Redundancies in the Spectral Domain
Source: arXiv:1305.1773 ancillary file (2013-05-27)
Supplement: Supplementary file 1 [file SupportingInformation.pdf]

# Sensitivity Enhancement of (Hyper-)CEST Image Series by Exploiting Redundancies in the Spectral Domain

Jörg Döpfert, Christopher Witte, Martin Kunth, Leif Schröder

*Leibniz-Institut für Molekulare Pharmakologie, Robert-Rössle-Str. 10, 13125 Berlin, Germany*

# - Supporting Information -

## Contents

**1 Direct Xe NMR Spectrum** **ii**

**2 Full data sets** **iii**

2.1 PCA reconstruction of a 32 × 32 CEST data set . . . . . . . . . . . . . . . . . . . . iii

2.2 Sub-sampling of a 64 × 64 CEST data set . . . . . . . . . . . . . . . . . . . . . . . . iv

**3 Sub-sampling details** **iv**

3.1 Sampling pattern . . . . . . . . . . . . . . . . . . . . . . . . . . . . . . . . . . . . . . iv

3.2 Recontruction details . . . . . . . . . . . . . . . . . . . . . . . . . . . . . . . . . . . . v

**4 Correction for overlapping CEST resonances (‘spillover’)** **v**

# 1 Direct Xe NMR Spectrum

The direct NMR spectrum of the sample used throughout this study is shown in Fig. S1. Xe@Solution denotes free xenon in solution, Xe@Gas xenon in the gas phase, and Xe@Cage xenon inside the host molecule. Note that the Xe@Solution signal is much larger than the Xe@Cage signal, motivating the application of indirect detection with CEST. The different DMSO content in the inner and the outer compartment of the phantom (see Fig. 1b)) in the main text) changes the chemical shift of the Xe@Cage resonance in each of the two volumes, yielding Xe@Cage$_{\text{in}}$ at $\omega_{\text{in}}$ = 76.3 ppm and Xe@Cage$_{\text{out}}$ at $\omega_{\text{out}}$ =79.5 ppm. Thereby, two different CEST agents Xe@Cage$_{\text{in}}$ and Xe@Cage$_{\text{out}}$ can be 'simulated' [1]. Note that also the Xe@Solution peak separates into a single peak for each compartment. However, this had no significant influence on the CEST images, since the receiver bandwidth of the gradient echo readout was sufficiently large.

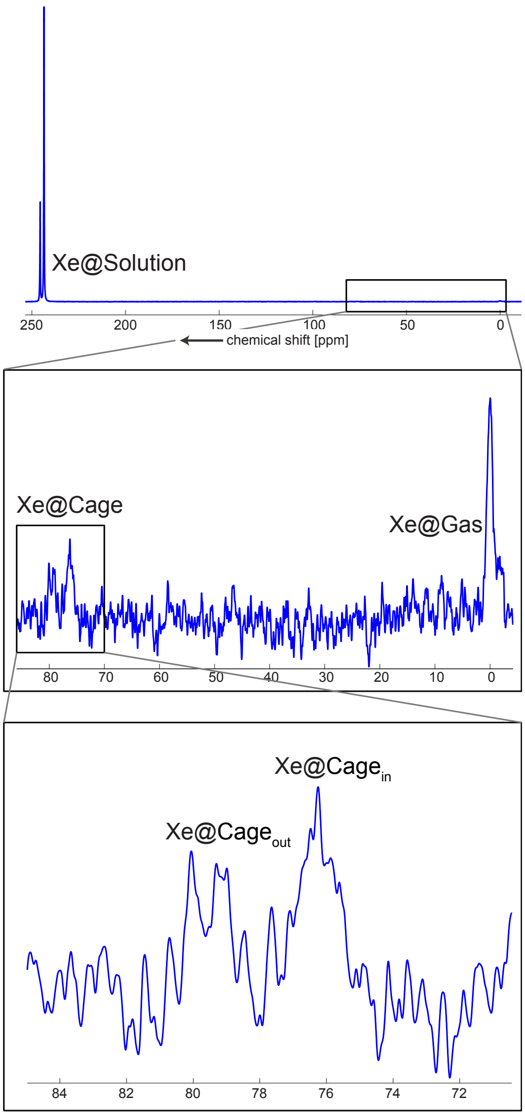


Figure S1: Xe NMR spectrum of the two compartment phantom acquired with a single pulse sequence (8 averages, 90 degrees excitation block pulse).

## 2 Full data sets

In this section, the full data sets containing all 17 CEST images are displayed.

### 2.1 PCA reconstruction of a $32 \times 32$ CEST data set

The full number of CEST images with and without PCA post-processing for the data set acquired with a $32 \times 32$ matrix is shown, corresponding to Fig. 2 in the main article.

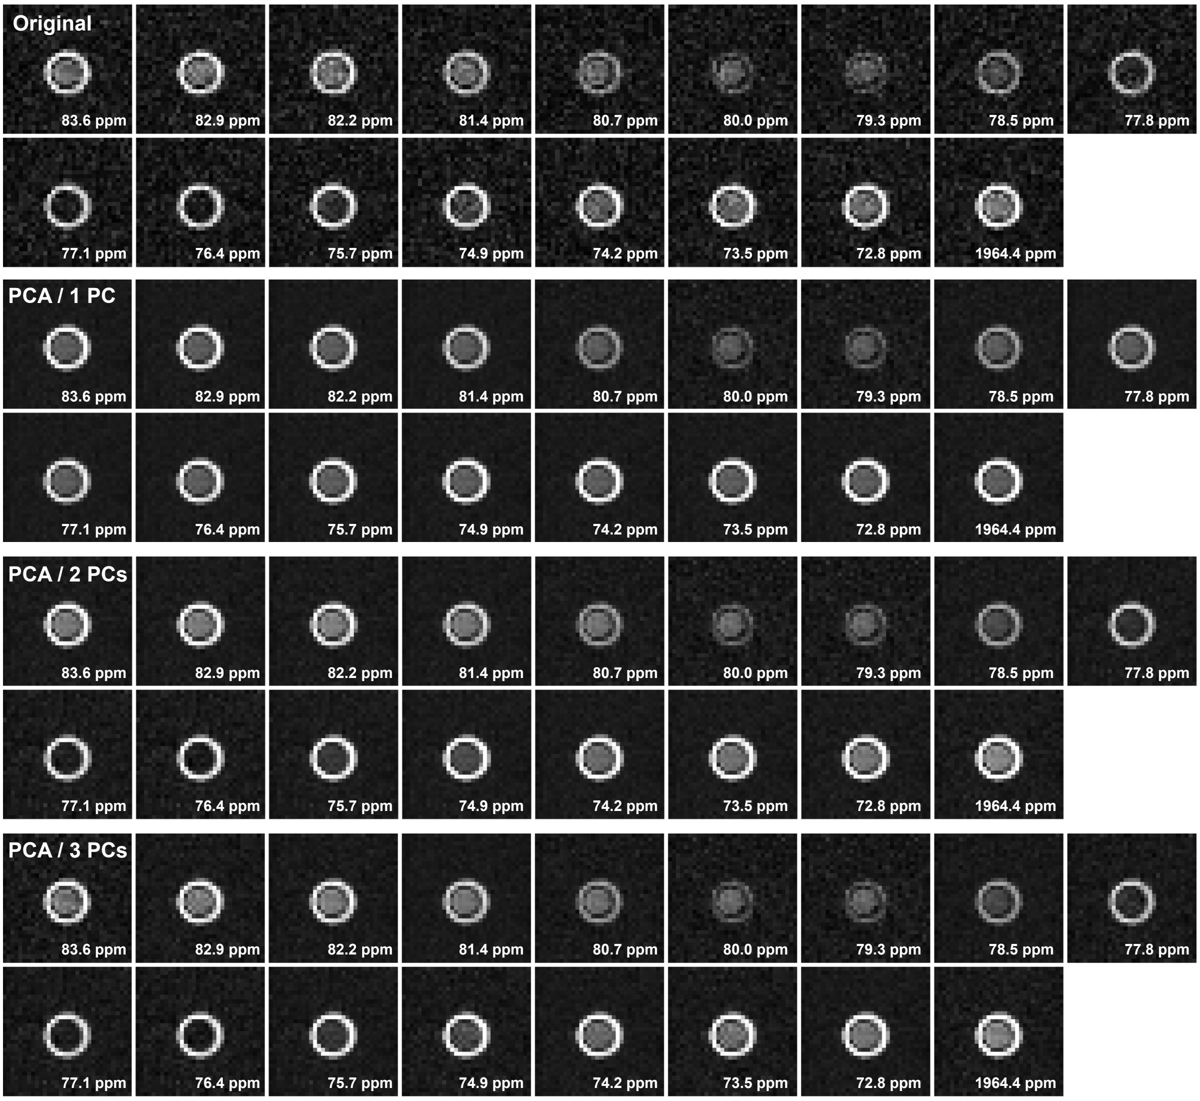


Figure S2: $32 \times 32$ data set corresponding to Fig. 2 of the main article: Original images and PCA post-processed images reconstructed using one, two and three of the highest ranked principal components (PCs). The reconstruction with only one PC does not correctly describe the saturation of the inner compartment (see image at 77.1 ppm), whereas the image series with two PCs already contains all the essential features of the data. Apparently no additional relevant information is obtained by including the third PC into the reconstruction.

### 2.2 Sub-sampling of a $64 \times 64$ CEST data set

The full number of CEST images for the data set from Fig. 3b) and c) in the main text is shown. Data were acquired with a $64 \times 64$ matrix, and both the fully sampled and the sub-sampled versions are depicted.

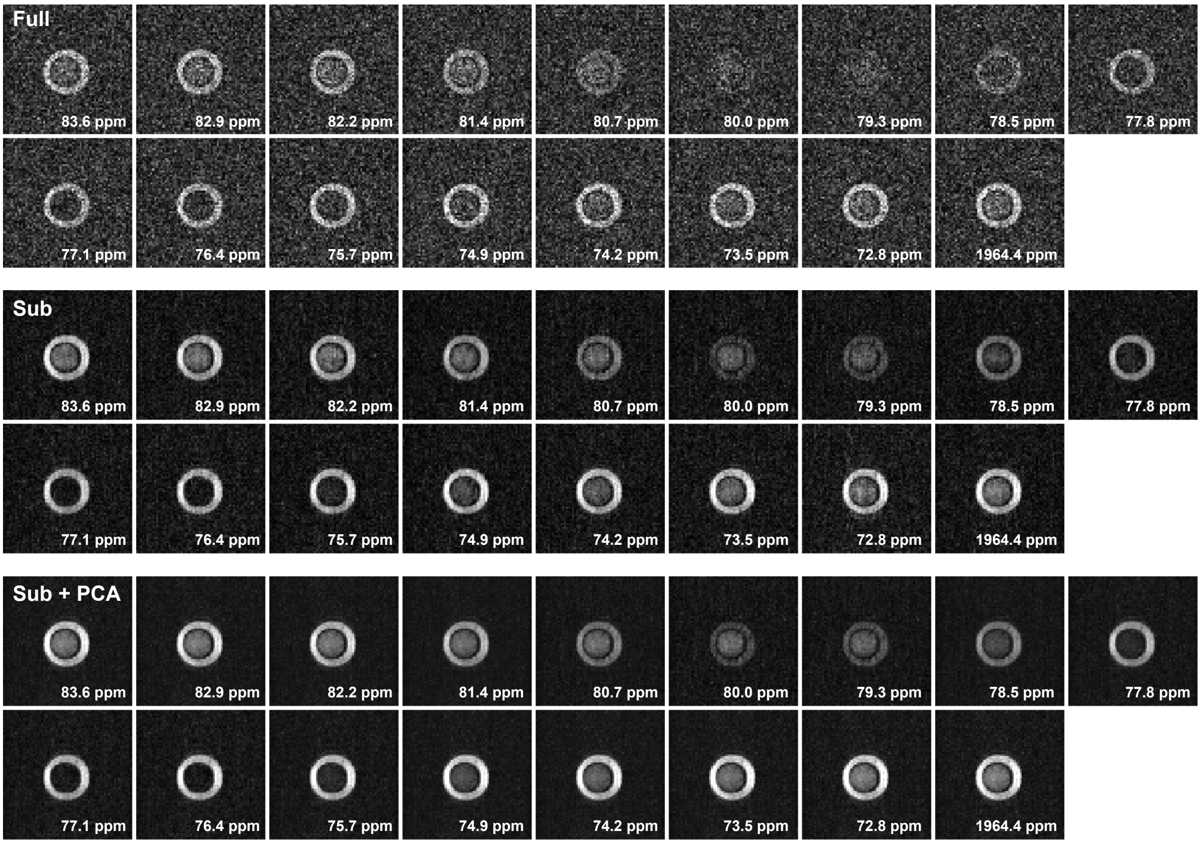


Figure S3: Top row: Fully sampled $64 \times 64$ CEST data set, corresponding to the top row of Fig 3c) in the main text. Middle row: Sub-sampled $64 \times 64$ data set, where only 34% of the data has been acquired, corresponding to the top row of Fig 3b) in the main text. Bottom row: The same data set as in the middle row, but this time post-processed using PCA with only the two highest ranked principal components, corresponding to the bottom row of Fig 3b).

## 3 Sub-sampling details

### 3.1 Sampling pattern

For each of the sub-sampled CEST data sets, $n_s = 22$ out of $n = 64$ phase encoding lines were acquired (34%). From these 22 lines, $n_c = 9$ were used to cover the center of $k$-space, and 13 lines were distributed in a pseudo-random fashion among remaining $k$-space. We acquired data sets with different values for $n_c$, and determined empirically that the ones $n_c = 9$ resulted in best image quality. We also compared the reconstructions for different $n_s$. Again, we determined by trial and error that only reconstructions with $n_s > 21$ exhibited no significant artefacts. A more correct analysis of the optimal sampling for a given undersampling factor is beyond the scope of this paper, since it is mainly supposed to demonstrate the applicability and benefit of sub-sampling regarding spectral CEST images.

We generated and tried out several pseudo-random distributions of the 13 non-central lines. Note that not all pseudo-randomly generated patterns can be used for image reconstruction: For example if a certain $k$-space line is not acquired at all in either of the CEST images, the low-rank reconstruction will not be able to provide an estimate about this line. The pattern we finally chose for all of our sub-sampled CEST images contains each $k$-space line at least once and is shown in Fig. S4. It cannot be completely ruled out the this pattern is in some sense "optimal" for the specific geometry of the phantom that we used. However, we consider this unlikely, since the 9 central lines that were always acquired already account for the main structure in the image.

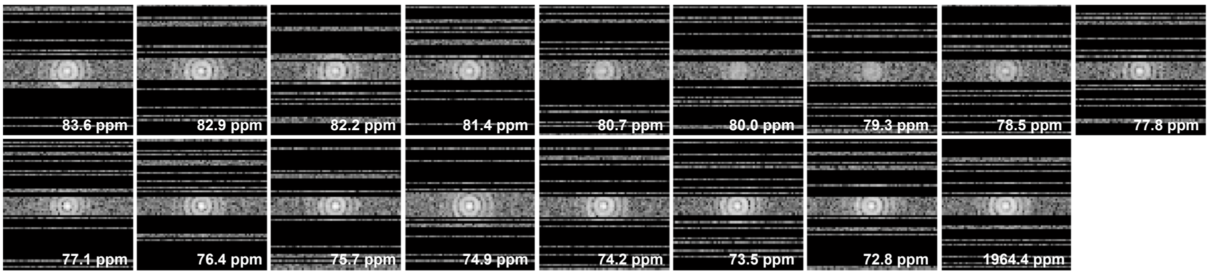


Figure S4: $k$-space of the sub-sampled image series to illustrate the sampling pattern. The pixel intensities are log-scaled, so that also data points from the outer regions of $k$-space are visible. Lines that have not been acquired are depicted in black (zero-filled).

### 3.2 Recontruction details

We run the Matlab implementation of the singular value thresholding algorithm (see file `SVT.m` from ref. [2]) on the $k$-space data of each sub-sampled 3D CEST data set, reshaped to a 2D matrix as described in section 2.1 of the main text. The parameters used in the reconstruction were: `delta` = 2 (stepsize), `tol` = 0.04 (tolerance), `tau` = 300000 (weighting factor for minimizing the nuclear norm, see ref. [3]). The `SVT` command returns three matrices, $\mathbf{U}$, $\mathbf{S}$ and $\mathbf{V}$, from which the reconstruction in image space was obtained by reshaping $\mathbf{USV}^*$ back into 3D form and then Fourier transforming it.

One might wonder why rank minimization was performed on the $k$-space data, since the discussion about redundancy and singular values in section 3 of the main text was all about image space. However, both spaces are equivalent in the sense that the rank of a data set in image space is the same as the rank in $k$-space due to injectivity of Fourier transform.

## 4 Correction for overlapping CEST resonances ('spillover')

This section shows that if the two CEST resonances to be detected overlap, four instead of three CEST images are required to correctly determine the CEST effect of each agent separately. For the moment, consider only the green curve in Fig. S5, assuming only one CEST agent (agent 1). Then the CEST effect can be calculated by taking the difference between an image acquired off-resonant (with negligible saturation) $\mathbf{S}_{\text{off}}$ at frequency $\omega_{\text{off}}$, and an image with maximum saturation $\mathbf{S}_{\text{on1}}$, saturating on-resonant at $\omega_1$. However, if a second CEST agent is present (agent 2, blue curve in Fig. S5), then the saturation pulse at $\omega_1$ will also partly saturate this second CEST agent (red arrow). The difference $\mathbf{S}_{\text{off}} - \mathbf{S}_{\text{on1}}$ will now have contributions from both CEST agents, making it impossible to discriminate between the two. To correct for this 'spillover', instead of the off-resonant image, another image $\widetilde{\mathbf{S}}_{\text{off1}}$ has to be acquired saturating

at a frequency $\widetilde{\omega}_1$ that is the reflection of $\omega_1$ around the frequency of the second agent, $\omega_2$. When assuming that the resonances of the CEST agents are symmetrical, agent 2 will contribute the same amount of saturation to $\widetilde{\mathbf{S}}_{\text{off1}}$ as to $\mathbf{S}_{\text{on1}}$ (the light blue arrow has the same length as the red one in Fig. S5). Hence, it is ensured that the difference $\widetilde{\mathbf{S}}_{\text{off1}} - \mathbf{S}_{\text{on1}}$ only shows contributions from agent 1 since the contributions from agent 2 cancel out. Repeating the procedure for agent 2, in total four images instead of three are required to obtain the correct CEST effect for both of the agents. Furthermore, the CEST effect will be lower when compared to the case of non-overlapping CEST resonances, since the 'off-resonant' image $\widetilde{\mathbf{S}}_{\text{off1}}$ is already partly saturated by constributions from CEST agent 1 (yellow arrow in Fig. S5). This decreases the CEST difference and hence the CEST effect of agent 1, but does not lead to a wrong estimation of the agent's localization.

The spillover correction is commonly performed in proton CEST MRI as well, but not due to overlap of different agents, but because the RF saturation pulse usually not only saturates the CEST agent, but also partly the bulk water resonance.

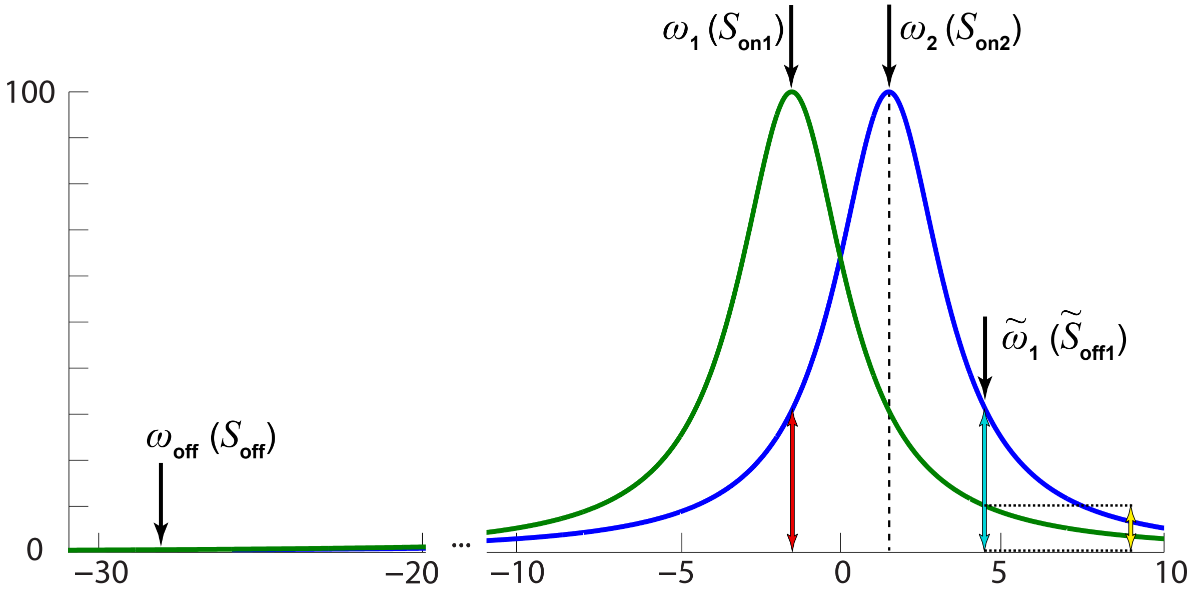


Figure S5: Schematic of overlapping resonances of two CEST agents for illustrating spillover correction.

## References


[1] Kunth M, Döpfert J, Witte C, Rossella F, Schröder L. Optimized use of reversible binding for fast and selective NMR localization of caged xenon. Angew. Chem. Int. Edit. 2012; 51: 8393. DOI: 10.1002/anie.201202481

[2] Singular Value Treshholding. http://www-stat.stanford.edu/∼candes/svt [1. August 2012]

[3] Cai JF, Candès EJ, Shen Z. A singular value thresholding algorithm for matrix completion. SIAM J. Optimiz. 2010; 20: 1956–1982. DOI: 10.1137/080738970
